# Supplementary material for: Implicit Neural Head Synthesis via Controllable Local Deformation Fields
Source: arXiv:2304.11113 source file (2023-04-21)
Supplement: Supplementary file 1 [file 05_misc.tex]

%\section{Negative Societal Impacts}
%{\color{red}The proposed method is formulated to help artists in their workflows. However, it can also be used maliciously to spread misinformation. However, our method has flaws that can be spotted as being synthetic.}
